# Supplementary material for: Dual Radar SAR Controller
Source: arXiv:2309.00006 source file (2023-06-27)
Supplement: Supplementary file 1 [file appendix01.tex]

\chapter{Multivariate Taylor Series Expansion}
\label{app:taylor_series_ffh}
