# Supplementary material for: Dual Radar SAR Controller
Source: arXiv:2309.00006 source file (2023-06-27)
Supplement: Supplementary file 2 [file appendix02.tex]

\chapter{Downloading the Toolbox}
\label{app:documentation}
